# Supplementary material for: A practical analysis of ROP attacks
Source: arXiv:2111.03537 source file (2021-11-05)
Supplement: Supplementary file 1 [file appendix.tex]

\clearpage
\section{Appendix}
\label{app:A}
...
